# Supplementary material for: Adversarial Robustness in Multi-Task Learning: Promises and Illusions
Source: arXiv:2110.15053 source file (2021-10-26)
Supplement: Supplementary file 1 [file _supplementary.tex]

\section{Appendix A: Proofs}

\section{Appendix B: Experimental Settings}

\section{Appendix C: Detailed evaluation of the factors}

\section{Appendix D: Qualitative Evaluation}

\subsection{Clean performances of each setting}

\subsection{Impact of the different architectures on all tasks}

\subsection{Impact of the different epochs on all tasks}

\subsection{W-PGD algorithm}

\begin{table*}
\caption{The experimental settings we evaluated.}
\label{experimental-settings}
\vskip 0.15in
\begin{center}
\begin{small}
%\begin{sc}
\begin{tabular}{llllllll}
\hline
 Setting & Dataset & Encoder & Loss & Tasks Decoder & \#Models & Training Epochs & Purpose  \\
\hline
 %S1 & Face &  M1 & Mono & (g,r) & 2 & & Baseline \\
 %S2 & Face &  M1 & Equal & (g,r) & 2 & & Task Sharing ** \\
 %S3 & Face &  M2 & Equal & (g,r) & 2 & & Task Sharing  ** \\
 S4 & Taskonomy &  Resnet18 & Mono & (s,d,D,n,k,K,e,E,p,r,A) & 11 & 150 & Baseline *\\
 S5 & Taskonomy &  Resnet50 & Mono & (s,d,D,n,k,K,e,E,p,r,A) & 11 & 150 & Baseline *\\
 S6 & Taskonomy &  Xception & Mono & (s,d,D,n,k,K,e,E,p,r,A) & 11 & 150 & Baseline \\
  S5 & Taskonomy &  Resnet152 & Mono & (s,d,D,n,k,K,e,E,p,r,A) & 11 & 150 & Baseline *\\
 S6 & Taskonomy &  Wide-resnet50 & Mono & (s,d,D,n,k,K,e,E,p,r,A) & 11 & 150 & Baseline \\
 
 S7 & Taskonomy &  Resnet18 & Equal & (s,d,D,n,k,K,e,E,p,r,A) & 110 & 150 & Attack Strategy **\\
 S8 & Taskonomy &  Resnet50 & Equal & (s,d,D,n,k,K,e,E,p,r,A) & 110 & 150 & Network Size *\\
 S9 & Taskonomy &  Xception & Equal & (s,d,D,n,k,K,e,E,p,r,A) & 110 & 150 & Architecture \\
  S8 & Taskonomy &  Resnet152 & Equal & (s,d,D,n,k,K,e,E,p,r,A) & 110 & 150 & Network Size *\\
 S9 & Taskonomy &  Wide-resnet50 & Equal & (s,d,D,n,k,K,e,E,p,r,A) & 110 & 150 & Architecture \\
 S10 & Taskonomy &  Resnet18 & Weighted & (s,d,D,n,k,K,e,E,p,r,A) & 110 & 150 & Task weighing *\\
 S11 & Taskonomy &  Resnet18 & Equal & (s,d,D,n,k,K,e,E,p,r,A) & 110 & 50 & Training epochs *\\
 S12 & Taskonomy &  Resnet18 & Equal & (s,d,D,n,k,K,e,E,p,r,A) & 110 & 100 & Training epochs *\\
% S11 & Taskonomy &  Resnet50 & Weighted & (s,d,D,n,k,K,e,E,p,r,A) & 110 \\
% S12 & Taskonomy &  Xception & Weighted & (s,d,D,n,k,K,e,E,p,r,A) & 110 \\
 
\hline
\end{tabular}
%\end{sc}
\end{small}
\end{center}
\vskip -0.1in
\end{table*}

\subsection{Clean performances of each setting}

\begin{table*}[]
\caption{MT task learning affinity.}
\label{learning-affinity}
\vskip 0.15in
\begin{center}
\begin{small}
\begin{tabular}{cccccccccccc}
\hline
Setting  & s & d & D & n & k & K & e & E & p & r & A  \\
\hline
 S4 & - & 0.0053 & 0.0052 & 0.0004 & 5.5302e-5 & 0.0014 & 0.0020 & 2.2380e-5 & 0.0034 & 0.0022 & 2.8164e-5\\
 S5 &  &  &  &  &  &  &  &  &  &  & \\
 S6 &  &  &  &  &  &  &  &  &  &  & \\
 S7 &  &  &  &  &  &  &  &  &  &  & \\
 S8 &  &  &  &  &  &  &  &  &  &  & \\
 S9 &  &  &  &  &  &  &  &  &  &  & \\
 S10 &  &  &  &  &  &  &  &  &  &  & \\
 S11 &  &  &  &  &  &  &  &  &  &  & \\
 S12 &  &  &  &  &  &  &  &  &  &  & \\
\hline
\end{tabular}
\end{small}
\end{center}
\vskip -0.1in
\end{table*}

\subsection{Clean performances of each setting}

\subsection{Size \& Complexity}

Xception27: 4.32M params  3.63B operation
Resnet18: 14.8 M params 6.09B operations
Resnet50: 29.66M params 9.89B operations
%\subsection{Statistical tests}

\begin{table}[t]
\caption{Statistical test of difference between Multi-task attack \& mono-task attack. Columns measured task.}
\label{stats-atks}
\vskip 0.15in
\begin{center}
\begin{small}
\begin{tabular}{cccccccccccc}
\hline
  & s & d & D & n & k & K & e & E & p & r & A  \\
\hline
 effect size &  &  &  &  &  &  &  &  &  &  & \\
 p-value &  &  &  &  &  &  &  &  &  &  & \\
\hline
\end{tabular}
\end{small}
\end{center}
\vskip -0.1in
\end{table}

\begin{table*}
\label{stats-atks}
\vskip 0.15in
\begin{center}
\begin{small}
\begin{tabular}{cc|ccccc|ccccc|ccccc|}
\hline
Attack &  & \multicolumn{5}{c|}{Vanilla (A)} & \multicolumn{5}{c|}{W-PGD Diff (B)} & \multicolumn{5}{c|}{Weighted Diff (C)}\\
\hline
     & & s & d & D & n & E & s & d & D & n & E& s & d & D & n & E  \\
\hline
\multirow{5}{*}{Mono} &s & \textit{0.82} & 0.86 & 0.97 & 0.96 & 0.93 & $>$0 & \textbf{$<$0} & 0.01 & 0.01 & 0.01 & $<$0 & 0.07 & -0.08 & -0.01 & -0.14 \\
& d & 5.74\textbf & \textit{5.61} & \textbf{5.28} & 6.88 & 6.41 & 1.6 & 0.02 & 1.8 & 2.98 & 3.22 & -0.48 & $>$0 & 0.36 & -2.08 & -0.9 \\
& D & \textbf{5.93} & \textbf{6.14} & \textit{6.4} & 7.12 & 8.31 & 1.66 & 2.38 & 0.02 & 3.05 & 3.04 & -0.58 & 0.25 & $<$0 & -1.32 & -1.59 \\
& n & \textbf{7.43} & \textbf{9.48} & \textbf{8.93} & \textit{10.82} & \textbf{9.08} & 1.67 & 3.16 & 2.36 & 3.34 & 3.26 & 1.9 & 2.89 & 1.14 & -0.01 & 0.65 \\
& E & \textbf{12.93} & \textbf{19.29} & \textbf{18.44} & \textbf{15.16} & \textit{22.57} & 0.02 & 0.03 & 0.01 & 0.01 & \textbf{-0.19} & 1.66 & -0.3 & 1.91 & -1.46 & 0.03 \\
\hline
  \multirow{5}{*}{Multi} &s & - & 0.85 & 0.96 & 0.95 & 0.91 & - & \textbf{-0.03} & \textbf{-0.03} & \textbf{-0.01} & \textbf{-0.01} & - & 0.06 & -0.08 & -0.04 & -0.15  \\
& d & \textbf{1.99} & - & \textbf{5.42} & \textbf{4.8} & \textbf{4.46} & 2.65 & - & 0.02 & 2.86 & 2.25 & -0.2 & - & 0.4 & -0.82 & -0.66 \\
& D & \textbf{2.14} & \textbf{6.02} & - & \textbf{5.02} & 6.07 & 2.46 & 0.03 & - & 2.55 & 2.68 & -0.28 & 0.15 & - & -0.7 & -0.75 \\
& n & \textbf{4.61} & \textbf{9.4} & \textbf{8.93} & - & \textbf{8.7} & 1.07 & \textbf{-3.33} & \textbf{-2.84} & - & \textbf{-0.55} & 0.79 & 2.7 & 1 & - & -0.72 \\
& E & \textbf{7.58} & \textbf{18.5} & \textbf{17.44} & \textbf{12.48} & - & 2.46 & \textbf{-6.11} & \textbf{-5.83} & 1.13 & - & 0.29 & -0.6 & 1.25 & -1.62 & - \\
\hline
\end{tabular}
\vskip -0.1in
\caption{Relative Task Robustness under different settings}
\end{small}
\end{center}
\end{table*}

\begin{table*}
\label{stats-atks}
\vskip 0.15in
\begin{center}
\begin{small}
\scalebox{0.8}{
\begin{tabular}{cc|ccccc|ccccc|ccccc|}
\hline
Attack &  & \multicolumn{5}{c|}{Vanilla (A)} & \multicolumn{5}{c|}{W-PGD (B)} & \multicolumn{5}{c|}{Weighted Diff (C)}\\
\hline
     & & s & d & D & n & E & s & d & D & n & E& s & d & D & n & E  \\
\hline
\multirow{5}{*}{Mono} &s & \textit{0.82} & 0.86 & 0.97 & 0.96 & 0.93 & \textit{0.82} & \underline{0.86} & 0.97 & 0.97 & 0.94 & $<$0 & 0.07 & -0.08 & -0.01 & -0.14 \\
& d & 5.74 & \textit{5.61} & \textbf{5.28} & 6.88 & 6.41 & 7.34 & \textit{5.63} & 7.09 & 9.86 & 9.63 & -0.48 & $>$0 & 0.36 & -2.08 & -0.9 \\
& D & \textbf{5.93} & \textbf{6.14} & \textit{6.4} & 7.12 & 8.31 & 7.59 & 8.53 & \textit{6.42} & 10.16 & 11.35 & -0.58 & 0.25 & $<$0 & -1.32 & -1.59 \\
& n & \textbf{7.43} & \textbf{9.48} & \textbf{8.93} & \textit{10.82} & \textbf{9.08} & \textbf{9.1} & \textbf{12.64} & \textbf{11.29} & \textit{14.16} & \textbf{12.35} & 1.9 & 2.89 & 1.14 & -0.01 & 0.65 \\
& E & \textbf{12.93} & \textbf{19.29} & \textbf{18.44} & \textbf{15.16} & \textit{22.57} & \textbf{12.95} & \textbf{19.32} & \textbf{18.45} & \textbf{15.17} & \underline{\textit{22.38}} & 1.66 & -0.3 & 1.91 & -1.46 & 0.03 \\
\hline
  \multirow{5}{*}{Multi} &s & - & 0.85 & 0.96 & 0.95 & 0.91 & - & \underline{0.81} & \underline{0.92} & \underline{0.94} & \underline{0.9} & - & 0.06 & -0.08 & -0.04 & -0.15  \\
& d & \textbf{1.99} & - & \textbf{5.42} & \textbf{4.8} & \textbf{4.46} & \textbf{4.63} & - & \textbf{5.44} & 7.66 & 6.71 & -0.2 & - & 0.4 & -0.82 & -0.66 \\
& D & \textbf{2.14} & \textbf{6.02} & - & \textbf{5.02} & 6.07 & 2.46 & 0.03 & - & 2.55 & 2.68 & -0.28 & 0.15 & - & -0.7 & -0.75 \\
& n & \textbf{4.61} & \textbf{9.4} & \textbf{8.93} & - & \textbf{8.7} & \textbf{5.68} & \underline{\textbf{6.07}} & \underline{\textbf{6.09}} & - & \underline{8.16} & 0.79 & 2.7 & 1 & - & -0.72 \\
& E & \textbf{7.58} & \textbf{18.5} & \textbf{17.44} & \textbf{12.48} & - & \textbf{10.04} & \underline{\textbf{12.39}} & \underline{\textbf{11.61}} & \textbf{13.61} & - & 0.29 & -0.6 & 1.25 & -1.62 & - \\
\hline
\end{tabular}
}
\vskip -0.1in
\caption{Relative Task Robustness under different settings}
\end{small}
\end{center}
\end{table*}
